# Supplementary material for: Electron volt energy resolution with ptychography using a broadband continuum spectrum
Source: arXiv:2409.00703 source file (2025-09-29)
Supplement: Supplementary file 1 [file ArXivSupplementaryMaterial.pdf]

# Supplementary Material

## Sample preparation

The NMC-622 sample was prepared at the Karlsruhe Institute of Technology (KIT) in Germany. For the experiment an NMC particle was mounted on the top of a syringe needle using a FIB-SEM to position and mount the particle. The needle was placed on the top of the scanning motor, a 3 axis MarsPI300 piezo stage. The sample was scanned in fly scanning mode as described in Ref. [1].

## k-edge for different Ni oxidation states

We measured the dependency of the k-edge as a function of the Ni oxidation state. The measurements are shown in Figure 1.

## Experimental image resolution estimation via FRC

Two consecutive acquisitions produced the two independent datasets used for calculating the Fourier ring correlation. The correlation between the two half datasets was compared to a half-bit information threshold, using an implementation based on van Heel et al. [4]. The resolution is 200 nm, see Figure 2.

## Fly-scanning ptychography

In a standard ptychographic acquisition, the sample is scanned across the illumination in step-and-shot mode: the sample is moved and, after a settling time required for the scanning motors to stabilise, an image is recorded by the detector. On the contrary, in fly scanning ptychography, the sample is moved continuously across the illumination while the detector acquires the diffraction patterns. This method allows to minimise the overheads [2] and enabling ultra-fast scanning[1]. The blurring effect due to the continuous motion can be compensated by using modal decomposition [3].

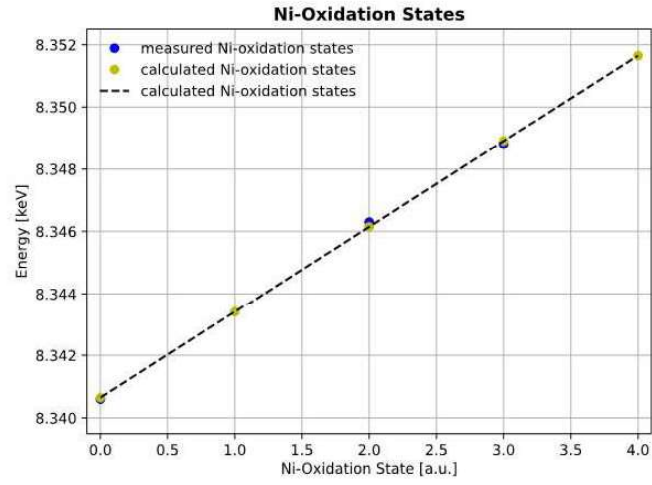

Figure 1: Measured k-edge variation as a function of the oxidation state.

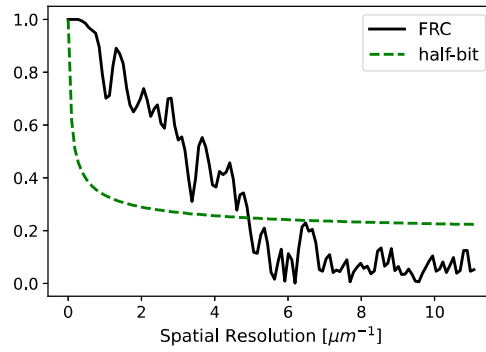

Figure 2: FRC for the 8.344 keV ptychographic reconstruction.

## References

- [1] D. Batey, C. Rau, and S. Cipiccia. High-speed x-ray ptychographic tomography. *Scientific Reports*, 12:7846, 2022.
- [2] P. M. Pelz, M. Guizar-Sicairos, P. Thibault, I. Johnson, M. Holler, and A. Menzel. On-the-fly scans for X-ray ptychography. *Applied Physics Letters*, 105(25):251101, 12 2014.
- [3] P. Thibault and A. Menzel. Reconstructing state mixtures from diffraction measurements. *Nature*, 494:68–71, 2013.
- [4] M. van Heel and M. Schatz. Fourier shell correlation threshold criteria. *Journal of Structural Biology*, 151(3):250–262, 2005.
